# Supplementary material for: Neural-Symbolic Reasoning over Knowledge Graphs: A Survey from a Query Perspective
Source: arXiv:2412.10390 source file (2026-08-22)
Supplement: Supplementary file 1 [file 009appendix.tex]

\noindent \textbf{Reproducibility.} All experiments are performed on a machine with an Intel(R) Xeon(R) Gold 6240R CPU, 1510GB memory and NVIDIA-SMI Tesla V100-SXM2. The details of datasets, machine and parameters can be found in Section ~\ref{experiments}. 
All datasets are publicly available. The source code of this paper can be found at \url{https://github.com/lihuiliullh/BiNet}.

\noindent \textbf{Baselines.}The implementation code of GraftNet, Key-Value Memory Network and EmbedKGQA can be found from the Table below. Because the source code of PullNet is not publicly available. We obtain its results from ~\cite{graftnet}. 

\begin{table}[h]
	\centering
	\caption{Baseline Source.}
	\small
	\begin{tabular}{|c|c|c|c|c|c|c|}
	\hline
	Model   & github \\ \hline
	GraftNet & {https://github.com/haitian-sun/GraftNet} \\ \hline
	KV-Mem & \url{https://github.com/jojonki/key-value-memory-networks} \\ \hline
	EmbedKGQA & \url{https://github.com/malllabiisc/EmbedKGQA} \\ \hline
	\end{tabular}
	\label{baseline_source}
\end{table}

For the knowledge graph completion baselines, we use LibKGE \url{https://github.com/uma-pi1/kge}. The training and testing configure file can be found from the repository.

\noindent \textbf{Dataset.}All the datasets used in this paper are publicly available which could be found in the Table below.

\begin{table}[h]
	\centering
	\caption{Dataset Source.}
	\small
	\begin{tabular}{|c|c|c|c|c|c|c|}
	\hline
	Model   & github \\ \hline
	MetaQA & \url{https://github.com/malllabiisc/EmbedKGQA} \\ \hline
	Webqsp & \url{https://github.com/malllabiisc/EmbedKGQA} \\ \hline
	SimpleQA & \url{https://github.com/davidgolub/SimpleQA/tree/master/datasets} \\ \hline
	\end{tabular}
	\label{dataset_source}
\end{table}

Table ~\ref{datasets} and Table ~\ref{datasets2} show the details of the datasets. Table ~\ref{datasets_30} shows the background knowledge graph used in the experiment which contains 70\% missing edges. The number of entities, number of relations and number of test edges are the same as 50\% incomplete knowledge graph. However, the number of train edges is much smaller.

\begin{table}
	\centering
	\caption{Summary of datasets. Coverage is the accuracy of subgraph matching. As we can see, simply applying edge traverse on the complete knowledge graph could achieve nearly 100\% accuracy.}
	\vspace{-1\baselineskip}
	\begin{tabular}{|c|c|c|c|c|c|c|}
	\hline
	Dataset          & Train & Valid & Test & Coverage \\ \hline
	{\tt MetaQA 1-hop} & 96,106   & 9,992     & 9,947  & 100\% \\ \hline
	{\tt MetaQA 2-hop} & 118,948   & 14,872       & 14,872 & 100\%  \\ \hline
	{\tt MetaQA 3-hop} & 114,196   & 14,274       & 14,274  & 99\% \\ \hline
	{\tt WebQSP} & 2,950   & -       & 1,560  & 99\%\\ \hline
	{\tt SimpleQA} & 15,3188   & 2,105       & 4,345 & 99\% \\ \hline
	\end{tabular}
	\label{datasets}
\end{table}

\begin{table}
	\centering
	\caption{Statistics of the 50\% KG for the three datasets. Note that WebQSP and SimpleQA use the same background knowledge graph.}
	\vspace{-1\baselineskip}
	\begin{tabular}{|c|c|c|c|c|c|c|}
	\hline
	Dataset          & Entities & Relations &  Train Edges & Test Edges \\ \hline
	{\tt MetaQA} & 43,234   & 18     & 66,791  & 4,000 \\ \hline
	{\tt WebQSP} & 1,886,683   & 1,144       & 2,872,880 & 20,000  \\ \hline
	{\tt SimpleQA} & 1,886,683   & 1,144       & 2,872,880  &  20,000 \\ \hline
	\end{tabular}
	\label{datasets2}
\end{table}

\begin{table}[h]
	\centering
	\caption{Statistics of the 30\% KG for the three datasets. Note that WebQSP and SimpleQA use the same background knowledge graph.}
	\begin{tabular}{|c|c|c|c|c|c|c|}
	\hline
	Dataset          & Entities & Relations &  Train Edges & Test Edges \\ \hline
	{\tt MetaQA} & 43,234   & 18     & 40,074 & 4,000 \\ \hline
	{\tt WebQSP} & 1,886,683   & 1,144       & 1,764,663 & 20,000  \\ \hline
	{\tt SimpleQA} & 1,886,683   & 1,144       & 1,764,663  &  20,000 \\ \hline
	\end{tabular}
	\label{datasets_30}
\end{table}

\noindent \textbf{Training Parameters.} When training \myModel\ on MetaQA, we use embedding dimension 200 and batch size 128. The learning rate is set to 0.0005. For datasets Webqsp and SimpleQA, we set embedding dimension to 200 and batch size to 16. The learning rate is set to 0.00002.

\noindent \textbf{The Pseudocodes.} 
The pseudocodes of \myModel\ are listed below.

\begin{algorithm}[H] % algorithm begin
	\caption{Knowledge Graph Question Answering Training} % Algorithm title
	\label{kgqa_alg} % algorithm label
	\begin{algorithmic}[1]
		\STATE \textbf{Input:} knowledge graph $\mathcal{G}=(\mathcal{V}, \mathcal{R}, \mathcal{L})$, training dataset $\{Q, A_Q\}_{train}$, hyper parameter $k$
		\STATE \textbf{Training:}
		\STATE Obtain question embedding $\mathbf{Q}$ from pre-trained $\textrm{BERT}$
		\STATE Calculate scores for all entities by Answer Scoring Module
		\STATE Select \topk\  candidates $S$
		\STATE Decode question embedding $\mathbf{Q}$ to obtain path $P$
		\FOR {each $v_i \in S$}
		\STATE Concatenate topic entity $v_Q$, path $P$ and $v_i$
		\STATE Use Transformer to calculate the score of  $v_i$
		\ENDFOR
		\STATE \textbf{Return} sorted \topk\ candidates
	\end{algorithmic}
\end{algorithm}

\begin{algorithm}[H] % algorithm begin
	\caption{Knowledge Graph Completion Training} % Algorithm title
	\label{kgc_alg} 
	\begin{algorithmic}[1]
		\STATE \textbf{Input:} knowledge graph $\mathcal{G}=(\mathcal{V}, \mathcal{R}, \mathcal{L})$, training datasets $\{v_Q, P, A_Q\}_{train}$, $\{(h, r, t)\}_{train}$ for KGC, hyper parameter $k$
		\STATE \textbf{Training:}
		\STATE Pre-train shared entity and relation embedding by $\{(h, r, t)\}_{train}$
		\STATE Head = topic entity $v_Q$
		\FOR {each $r_i \in P$}
		\STATE Beam search according to Head and $r_i$
		\STATE Head = \topk\ candidates
		\ENDFOR
		\STATE \textbf{Return} the best sorted candidate
	\end{algorithmic}
\end{algorithm}
\vspace{-1\baselineskip}

\noindent \textbf{The Results of Path Decoder.} Table ~\ref{path_decoder} shows the results of the path decoder.

\begin{table*}
	\centering
	\caption{Results of Path Decoder.}
	\vspace{-1\baselineskip}
	\small
	\begin{tabular}{|c|c|}
	\hline
	Question       & Path \\ \hline
	the movies starred by [Tanner Maguire] were in which genres & starred\_actors\_reverse | has\_genre \\ \hline
	when did the movies written by [Cristian Nemescu] release  &  written\_by\_reverse | release\_year \\ \hline
	the films acted by [Benjamin Pitts] were released in which years   &  Starred\_actors\_reverse | release\_year \\ \hline
	who are movie co-writers of [Ray Ashley] & written\_by\_reverse | written\_by \\ \hline
	who co-starred with [Mary McDonnell]  &  starred\_actors\_reverse | starred\_actors \\ \hline
	who are movie co-directors of [Jack Hazan]  & directed\_by\_reverse | directed\_by \\ \hline
	%what genres do the movies directed by [Kevin Munroe] fall & directed\_by\_reverse | has\_genre \\ \hline
	\end{tabular}
	\label{path_decoder}
	\vspace{-1\baselineskip}
\end{table*}
